# Supplementary material for: LNS-Madam: Low-Precision Training in Logarithmic Number System using Multiplicative Weight Update
Source: arXiv:2106.13914 source file (2022-08-23)
Supplement: Supplementary file 1 [file additional_results.tex]

\subsection{Additional Results}
