# Supplementary material for: LNS-Madam: Low-Precision Training in Logarithmic Number System using Multiplicative Weight Update
Source: arXiv:2106.13914 source file (2022-08-23)
Supplement: Supplementary file 4 [file main_appendix.tex]

\documentclass{article}
%%%% official setting %%%%

% if you need to pass options to natbib, use, e.g.:
\PassOptionsToPackage{numbers, compress}{natbib}
% before loading neurips_2021

% ready for submission
\usepackage{template/neurips_2021}
\usepackage{icml2021/algorithm}
\usepackage{icml2021/algorithmic}
% to compile a preprint version, e.g., for submission to arXiv, add add the
% [preprint] option:
%     \usepackage[preprint]{neurips_2021}

% to compile a camera-ready version, add the [final] option, e.g.:
%     \usepackage[final]{neurips_2021}

% to avoid loading the natbib package, add option nonatbib:
%    \usepackage[nonatbib]{neurips_2021}

\usepackage[utf8]{inputenc} % allow utf-8 input
\usepackage[T1]{fontenc}    % use 8-bit T1 fonts
\usepackage{hyperref}       % hyperlinks
\usepackage{url}            % simple URL typesetting
\usepackage{booktabs}       % professional-quality tables
\usepackage{amsfonts}       % blackboard math symbols
\usepackage{nicefrac}       % compact symbols for 1/2, etc.
\usepackage{microtype}      % microtypography
\usepackage{xcolor}         % colors

%%%%  %%%%

%%%%% additional packages
%\usepackage{hyperref}
\usepackage{url}
\usepackage{multirow}

\usepackage{siunitx}
\sisetup{output-exponent-marker=\ensuremath{\mathrm{e}}}

% \usepackage{titlesec}
% \titlespacing*{\section}{0pt}{0.8\baselineskip}{\baselineskip}
\usepackage[compact]{titlesec}

% \usepackage{cite} planning to change
% \usepackage{natbib}
% \setcitestyle{square,comma,numbers}
% \bibliographystyle{abbrvnat}

% \setlength{\abovecaptionskip}{1pt}
% \setlength{\belowcaptionskip}{-8pt}
% \setlength{\belowdisplayskip}{0pt}
% \setlength{\belowdisplayshortskip}{0pt}
% \setlength{\abovedisplayskip}{0pt}
% \setlength{\abovedisplayshortskip}{0pt}
% \setlength{\textfloatsep}{2pt}
% \setlength{\floatsep}{6pt plus 1pt minus 0pt}
% \setlength{\intextsep}{3pt plus 1pt minus 0pt}
% \setlength{\dbltextfloatsep}{3pt plus 1pt minus 0pt}
% \setlength{\dblfloatsep}{3pt plus 1pt minus 0pt}
\linespread{0.96}
%
%\cfoot{\thepage}
\input{packages}
\input{macros}
\input{math_command}

% \PassOptionsToPackage{numbers,sort&compress}{natbib}

\begin{document}

% \input{sections/0-title}
% \maketitle
% \input{sections/1-abstract}
% \input{sections/2-intro}
% \input{sections/4-method}
% \input{sections/5-method}
% \input{sections/6-method}
% \input{sections/8-experiment}
% \input{sections/3-related}
% \input{sections/9-discussion}

% \bibliographystyle{unsrtnat}
% \bibliography{refs}
% \newpage
% \input{sections/10-checklist}

\appendix
\input{sections/X-theory}
\input{sections/X-hardware}
\input{sections/X-experiment}
\bibliographystyle{unsrtnat}
\bibliography{refs}

\end{document}
